# Supplementary material for: Labor Market Effects of the Venezuelan Refugee Crisis in Brazil
Source: arXiv:2302.04201 source file (2024-05-24)
Supplement: Supplementary file 1 [file border_analysis.tex]

So far we have explored the labor market effects of the Venezuelan refugee crisis at the state level and the capital municipality level. In this section, we examine the impact on the formal labor market of Pacaraima, the border municipality in Roraima located adjacent to Venezuela. Besides the capital, Boa Vista, Pacaraima was the municipality most affected by the crisis. Unlike Boa Vista, which has a more diverse local market, Pacaraima’s labor market is dominated by retail, with a considerable percentage of the population working in this economic sector. We employ the difference-in-differences specification explained in equation \ref{eq:wagesdid} to analyze whether the wage effects are different from our main results focused on the state capitals, given the difference in market size and diversity. We take the border municipalities in the control states, Acre and Amapa, as control units for comparison.

Table \ref{tab:border_results} displays the analysis results. Columns (1) to (3) include data from all 11 years used in the previous regression samples. The model with covariates and individual and year fixed effects shows that the Venezuelan crisis led to a nearly 5 percent decrease in wages for Brazilians in the border municipality. Figure \ref{fig:border_mainresults_es} plots the coefficients from the equivalent event study using equation \ref{eq:wageses}.

The event study figure shows that the parallel trends assumption is only weakly satisfied. To address this issue, we ran an alternative regression using a sample limited to 2010 and beyond. Columns 4 and 5 show the results of this restricted sample. The estimates are now smaller and have lost their significance. When using the balanced dataset, there is a 1.4 percent decrease in wages for Brazilians in Pacaraima compared to control state border municipalities.

Contrasting our results for the capital, the border municipality results showed no significant effect on the aggregate market, suggesting that the labor market was unable to benefit from labor complementarity. This may be due to the lack of diversity in occupations available in Pacaraima, as it is a smaller market. Therefore, we also show evidence that market diversity plays a role in determining the extent of labor complementarity in the face of an immigration supply shock, which future research should focus on.

\begin{table}[htb!]
    \vspace{1cm}
    \centering 
    \caption{Effects in the Border Municipality} \label{tab:border_results}
    \resizebox{0.85\textwidth}{!}{
\begin{tabular}[t]{lccccc}
\toprule
\multicolumn{1}{c}{} & \multicolumn{5}{c}{Log Wage} \\
\cmidrule(l{3pt}r{3pt}){2-6}
  & (1) & (2) & (3) & (4) & (5)\\
\midrule
Treated & \num{-0.050}* & \num{-0.050} & \num{-0.049} & \num{-0.038} & \num{-0.014}\\
 & (\num{0.025}) & (\num{0.024}) & (\num{0.024}) & (\num{0.027}) & (\num{0.019})\\
\midrule
Individual FE & X & X &  & X & X\\
Individual x Municipality FE &  &  & X &  & \\
Year FE & X & X & X & X & X\\
Covariates &  & X & X & X & X\\
Balanced Panel Data &  &  &  &  & X\\
Restricted Pre-Treatment Period &  &  &  & X & X\\
N & \num{40398} & \num{40398} & \num{40398} & \num{32736} & \num{18154}\\
\bottomrule
\multicolumn{6}{l}{\rule{0pt}{1em}\textsuperscript{1} Standard-errors are clustered by municipality.}\\
\multicolumn{6}{l}{\rule{0pt}{1em}\textsuperscript{2} Covariates are individual's race, age, age-squared, gender, and education level.}\\
\multicolumn{6}{l}{\rule{0pt}{1em}\textsuperscript{3} Restricted Pre-Treatment Period excludes 2007, 2008 and 2009}\\
\end{tabular}
}
\end{table}

\begin{figure}[h!]
\vspace{0.3cm}
\centering 
        \caption{Border Analysis Event Study} \label{fig:border_mainresults_es}
        \includegraphics[width=0.7\textwidth]{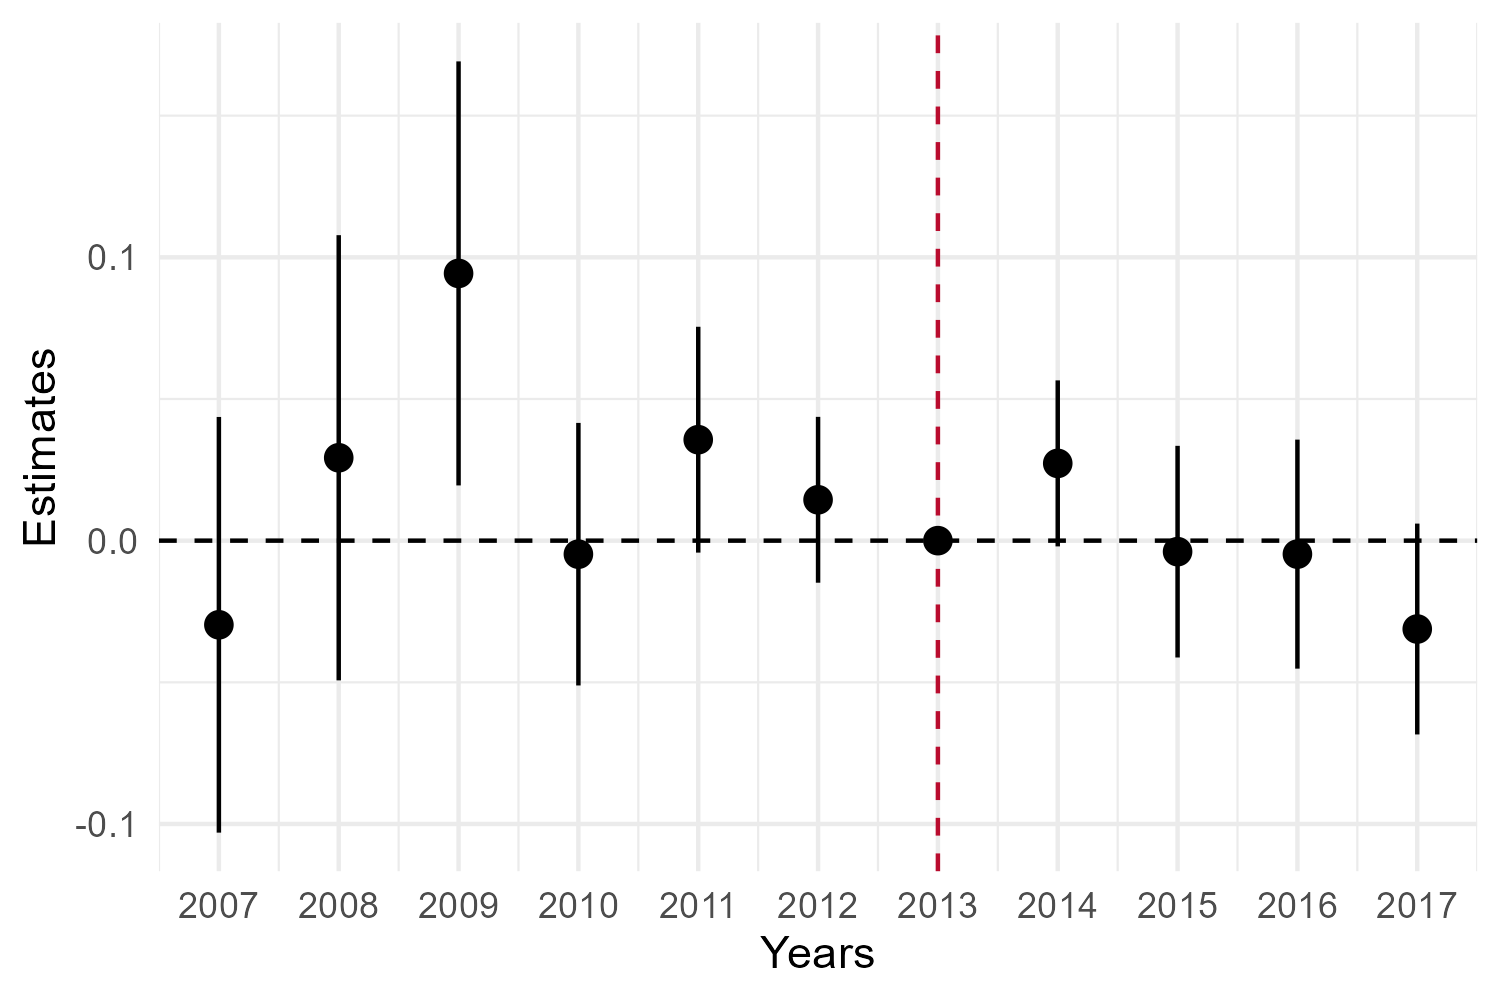}  
 \end{figure}
