# Supplementary material for: Labor Market Effects of the Venezuelan Refugee Crisis in Brazil
Source: arXiv:2302.04201 source file (2024-05-24)
Supplement: Supplementary file 2 [file conare.tex]

We rely on the identifying assumption that due to geographical setting, the Venezuelan refugees in Brazil enter through the state of Roraima and not in the control states. The RAIS dataset provides a good picture of this pattern, however, it only enumerates Venezuelans in the formal labor market. If the control states host a sizeable number of Venezuelan refugees who work in the informal labor sector, it will jeopardize our identification strategy. To show that it is not the case, we rely on the refugee application data from the National Committee for Refugees (CONARE).

Foreigners in Brazil can be registered as refugees to get benefits such as obtaining the individual taxpayer registration number (CPF), accessing health and education services, and other social benefits, and requesting the opening of a bank account, among others. An individual submits a request for the recognition of refugee status (via Sisconare and document insurance by the federal police). The applications are then analyzed by CONARE. The committee then decides whether an individual is recognized as a refugee. If they are not recognized as refugees, they can appeal for refugee status again.

The data provided by CONARE include the nationality of the applicants, the reason for leaving their country, the date when the application was submitted, the municipality and the state where the application was submitted, and the date when the decision was made by CONARE.

Table \ref{fig:conare_trend} shows the cumulative number of refugee applications by treatment status and year between 2011 and 2020. There were 56,984 refugee requests in Roraima in the 10-year period, with the first application submitted in 2015. Conversely, there was a meager number of refugee requests in the control states at 164.

Combining Figure \ref{fig:conare_trend} and Table \ref{tab:vz_entries}, however, we find that only around 20 percent of the Venezuelan refugees in 2017 had applied for refugee status in Roraima. Among those who were granted refugee status, only around 1,500 entered the formal labor market. We can thus infer that a significant fraction of Venezuelan refugees should be working in the informal labor market.

% 1 out 4 applied refugee status. 10k out 40k (federal police data)
%10,000/40,000

% 30k we dont know what they are doing.

% 8k that sought for a job but didnt get a job in the formal sector
% 1.5k got a job in the formal sector

\begin{figure}[htb!]
    \centering
    \includegraphics[width =0.8\textwidth]{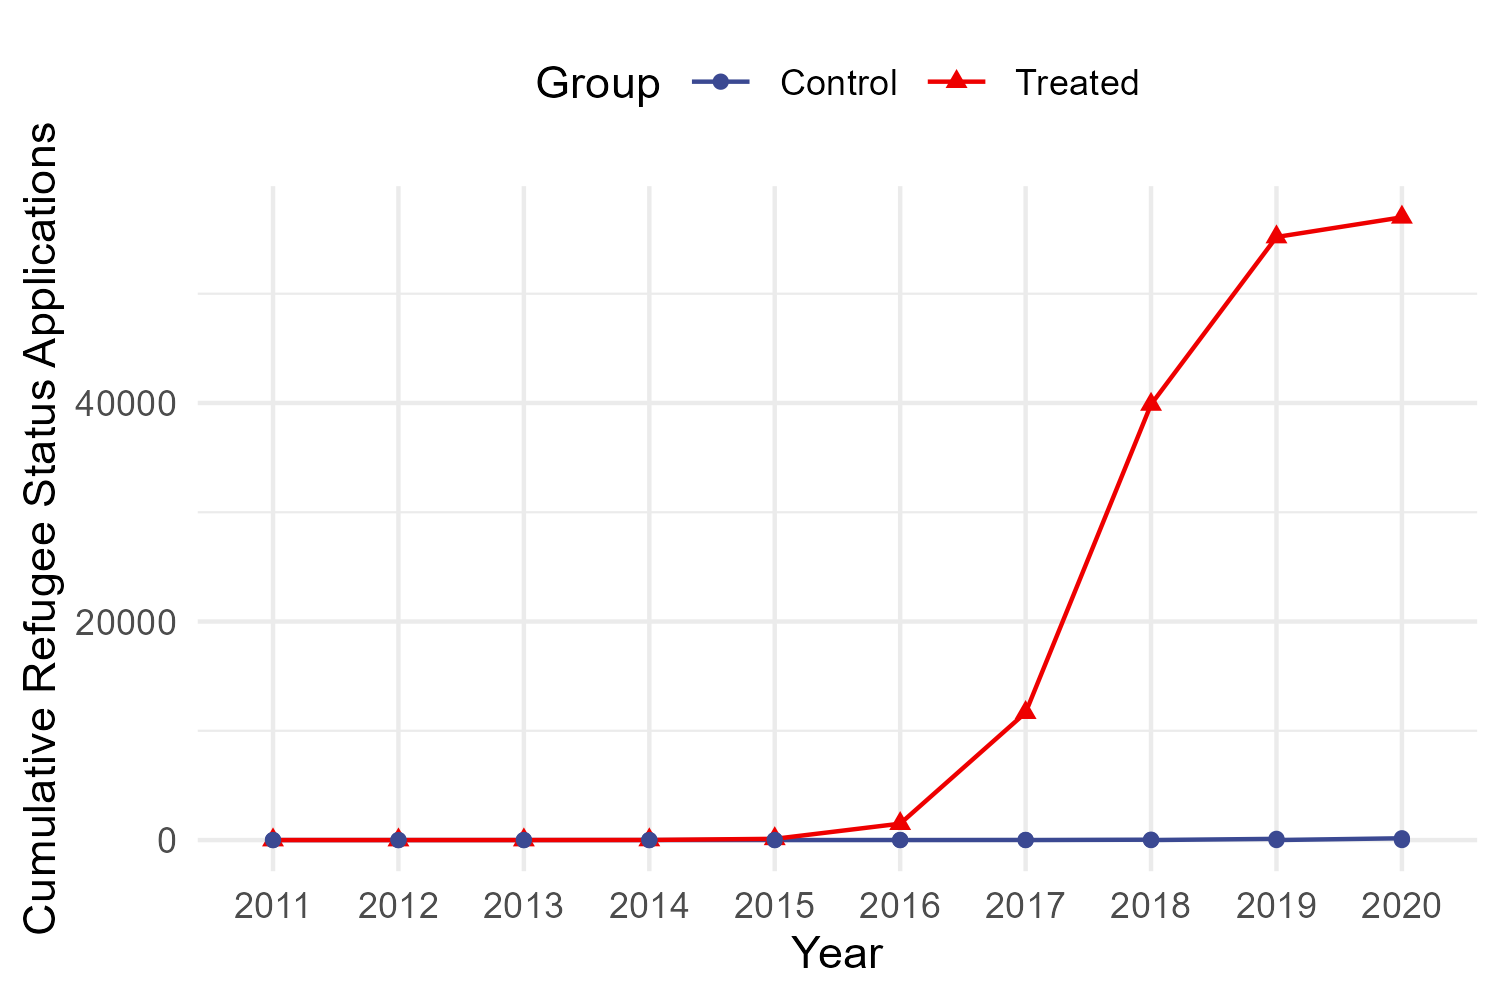}
    \caption{Cumulative refugee requests by year and treatment status}
    \label{fig:conare_trend}
\end{figure}
