# Supplementary material for: Labor Market Effects of the Venezuelan Refugee Crisis in Brazil
Source: arXiv:2302.04201 source file (2024-05-24)
Supplement: Supplementary file 3 [file structuralmodel.tex]

Consider an economy with a single output good $Y$ produced by a representative firm with three imperfect substitute inputs:

\begin{equation}
    Y =  H^{\alpha} L^{\beta} I^{1 - \alpha - \beta}
\end{equation}

where $I$ represents the labor supply of informal workers, $L$ represents the labor supply of formal low-skilled workers, and $H$ represents the labor supply of formal high-skilled workers. $\alpha$ represents the preference for high-skilled workers, while $\beta$ represents the preference for formal low-skilled workers. Individuals working in the informal market possess the same skill level as formal low-skilled workers.

Let $\{w_i, w_l, w_h\}$ be the wages associated with informal, low-skilled, and high-skilled workers respectively. Hence, the firm maximizes its profits by optimizing

\begin{equation}
    \max_{H, L, I} H^{\alpha} L^{\beta} I^{1 - \alpha - \beta} -w_i I - w_l L - w_h H
\end{equation}

where $w_i < w_l < w_h$ and $0 < \alpha + \beta < 1$. The first-order conditions for this problem concerning labor supply can be written as:

\begin{align}
    w_i &= (1 - \alpha - \beta) \frac{Y}{I} \\
    w_l &= \beta \frac{Y}{L} \\
    w_h &= \alpha \frac{Y}{H} 
\end{align}

Let $\Bar{L}$ represent the labor supply of low-skilled individuals. They are allowed to supply both the informal and low-skilled formal sectors. Let $\Bar{H}$ represent the high-skilled labor supply. They can only work in high-skilled positions. The market clearing conditions can be written as:

\begin{align}
    \Bar{L} &= I + L \\
    \Bar{H} &= H
\end{align}

\subsection{Introducing the Immigrants}

We observe the vast majority of Venezuelans occupying manual-intensive jobs in the formal sector, represented by the $L$ in our equations. We do not observe the foreign informal workers in the market, however, we know the number of refugees in Roraima is much higher than their observed formal workers, with a significant portion requesting refugee status. Hence, we can conclude a noticeable fraction of this new population is at least willing to supply labor in the informal sector.

Let $\bar{L}'$ represent the low-skilled population after an immigration shock, where $\bar{L}' = (1 + \delta )\bar{L}$, with $0 < \delta < 1$ representing the fraction of immigrants in the population. We can write the new market clearing condition as follows:

\begin{align}
   \Bar{L}' = (1 + \delta)\Bar{L} &= (1 + \eta)L + (1 + \mu)I \\
   \Bar{H}' = \Bar{H} &= H
\end{align}

Where $\eta$ and $\mu$ correspond to the proportion of immigrants in the formal and informal sectors respectively. Our assumption $\mu > \eta$ represents the fact we observe only a small fraction of immigrants working in the formal sector in our data.

To calculate the new wages, we combine Equations B.3, B.4, B.5, B.8, and B.9:

\begin{align}
    w_i' &= w_i \frac{(1 + \eta)^\beta}{(1 + \mu)^{\alpha + \beta}}\\
    w_l' &= w_l \frac{ (1 + \mu)^{1 - \alpha - \beta}}{(1 + \eta)^{1 - \beta}} \\
    w_h' &= w_h (1 + \eta)^\beta (1 + \mu)^{1 - \alpha - \beta}
\end{align}

Since our parameters are strictly positive, it is clear that $w_h' > w_h$. It is also straightforward to conclude $w_i' > w_i$ as long as $\mu > \eta$. The immigration effect magnitude on low-skilled wages will depend on the market's preferences, reflecting our results as being indistinguishable from the null hypothesis.
