# Supplementary material for: Labor Market Effects of the Venezuelan Refugee Crisis in Brazil
Source: arXiv:2302.04201 source file (2024-05-24)
Supplement: Supplementary file 4 [file econ_activity_table.tex]

\resizebox{\textwidth}{!}{%
        \begin{tabular}{llc} \label{tab:cnaecategories}
           \tabularnewline\midrule\midrule
           First 2-digit code & Definition \\
           \midrule
           01...03 & Agriculture, livestock, hunting, and fishing related activities.\\
           05...09 & Extraction industry. \\
           10...33 & Transformation industry. \\
           35      & Gas and Electricity. \\
           36...39 & Water distribution and waste \\
           41...43 & Construction. \\
           45...47 & Commerce (retail and wholesale. We call retail and commerce interchangeably in this paper). \\
           49...53 & Transportation. \\
           55...56 & Restaurants and hotels. \\
           58...63 & Information and communication.\\
           64...66 & Financial activities, insurance. \\
           68      & Real state. \\
           69...75 & Research related activities.\\
           77...82 & Administrative services. \\
           84      & Public administration, defense and social security.\\
           85      & Education.\\
           86...88 & Human health and social services.\\
           90...93 & Arts, culture and sports.\\
           94...96 & Other economic activities.\\
           97      & Domestic services.\\
           99      & International organizations and other foreign institutions.\\
           \midrule
           \multicolumn{2}{l}{\rule{0pt}{1em}{\makecell[l]{\textsuperscript{1} Each digit in the coding system represents an additional level of detail for the economic activity \\ variable. For example, 01 stands for agriculture, livestock, forestry, and aquaculture. 01.5 stands \\ for livestock. If we go even further, 01.51-2 represents bovine livestock. 01.51-2/02 is the highest level, \\ representing bovine milk producers. For the purposes of this study, we used the first two digits of the code \\ to categorize a broader but still detailed economic activity.}}}
        \end{tabular}%
    }
