# Supplementary material for: Labor Market Effects of the Venezuelan Refugee Crisis in Brazil
Source: arXiv:2302.04201 source file (2024-05-24)
Supplement: Supplementary file 7 [file entries.tex]

\begin{tabular}{lccc} \label{tab:federalreport}
   \tabularnewline\midrule\midrule
        Year & Entry & Exit & Stayed\\
        \midrule
        2015 & 32294 & 28979 & 3315\\
        \midrule
        2016 & 57106 & 47429 & 9677\\
        \midrule
        2017 & 70757 & 29002 & 41755\\
   \midrule
\end{tabular}
